# Supplementary material for: Harnessing the Power of LLMs in Practice: A Survey on ChatGPT and Beyond
Source: arXiv:2304.13712 source file (2023-04-27)
Supplement: Supplementary file 1 [file Appendix.tex]

A short report of results from GPT-3, GTP-3.5, Palm, GPT-4, ChatGPT

\section{GPT-4}

1994 definition of intelligence: \emph{a very general mental capability that, among other things, involves
the ability to reason, plan, solve problems, think abstractly, comprehend complex ideas, learn quickly and learn from experience.}\footnote{Mainstream science on intelligence: An editorial with 52 signatories,
history, and bibliography, 1997.}

Problems:
\begin{itemize}
    \item hallucinations
    \item
\end{itemize}

\section{ChatGPT}

\section{GPT-3}
In the zero-shot setting, the model can rarely perform any of the tasks (Table 3.10). This suggests that the model really does appear to learn these tasks at test time, as the model cannot perform them zero-shot and their artificial nature makes them unlikely to appear in the pre-training data (although we cannot confirm this with certainty. 
(Word scambing)

\section{Palm}

The way of finetuning: to use the decoder-only architecture during finetuning, inputs and targets are
concatenated but loss is only computed in the target section of the sequence. The concatenated sequences
are truncated to 2048 tokens, the training context used during pretraining, with 512 tokens reserved for the
target. Only summarization tasks required input truncation.

\section{Bloom}

It discusses several translation prompts/instructions:

\begin{table}[]
    \centering
    \begin{tabular}{c|c}
       a_good_translation-source+target  &  Given the following source text: [source sentence], a good L2 translation is: & [target sentence] \\
       gpt3-target & What is the L2 translation of the sentence: [source sentence]? & [target sentence] \\
       version-target & if the original version says [source sentence]; then the L2 version should say:& [target sentence]\\
       xglm-source+target &  L1: [source sentence] = L2: & [target sentence]
    \end{tabular}
    \caption{Caption}
    \label{tab:translation}
\end{table}
